# Supplementary material for: Intrinsic subthermionic capabilities and high performance of easy-to-fabricate monolayer metal dihalide MOSFETs
Source: arXiv:2106.12077 ancillary file (2021-06-22)
Supplement: Supplementary file 1 [file Supplemetary_Material.pdf]

# Intrinsic subthermionic capabilities and high performance of easy-to-fabricate monolayer metal dihalide MOSFETs

D. Logoteta, J. Cao, M. Pala, P. Marconcini, and G. Iannaccone

# Supplementary Information

## S1. Derivation of Eq (1) of the main text

The Laundauer's formula reads [1]:

$$I_{DS} = \frac{2q_e}{h}\int_{-\infty}^{\infty} dE\ \mathcal{T}(E)\ D(E)[f(E - E_{FS}) - f(E - E_{FD})], \qquad (1)$$

where $\mathcal{T}$ is the transmission, $D$ is the density of states, $f$ is the Fermi-Dirac distribution, $E$ is the energy, $E_{FS}$ and $E_{FD}$ are the Fermi levels at the source and drain contacts, respectively, $q_e$ is the electron charge and $h$ is Planck's constant. The previous formula can be simplified by assuming $E_{FS} = 0$ and approximating $f(E - E_{FS}) - f(E - E_{FD}) \approx f(E - E_{FS})$. We also approximate the transmission as $\mathcal{T}(E) \propto \Theta(E - \Phi_B)$, where $\Theta(E)$ is the Heaviside function and $\Phi_B$ is the height of the channel barrier with respect to $E_{FS}$. This approximation is valid when the gate of the transistor is long enough to make source-to-drain tunnelling negligible. Under these hypotheses Eq. (1) can be rewritten as:

$$I_{DS} \propto \frac{2q_e}{h}\int_{\Phi_B}^{\infty} dE\ D(E)\, e^{-\frac{E}{KT}} = \frac{2q_e}{h}\left[KTe^{-\frac{\Phi_B}{KT}}D(\Phi_B) + KT\int_{\Phi_B}^{\infty} dE\ \ e^{-\frac{E}{KT}}\frac{\partial D(E)}{\partial E}\right],$$

where the last equality is obtained by expanding the integral by parts.

According to the definition, the subthreshold swing is finally computed as

$$SS = \left(\frac{\partial \log_{10} I_{DS}}{\partial V_G}\right)^{-1} = \frac{1}{q_e}\left(\frac{\partial \log_{10} I_{DS}}{\partial \Phi_B}\right)^{-1}\left(-\frac{\partial \Phi_B}{\partial (q_e V_{GS})}\right)^{-1}$$

$$= \frac{KT}{q_e}\ln(10)\left(-\frac{\partial \Phi_B}{\partial (q_e V_{GS})}\right)^{-1}\left(1 + \frac{\int_{\Phi_B}^{\infty} dE\ \ e^{-\frac{E}{KT}}\frac{\partial D(E)}{\partial E}}{e^{-\Phi_B/KT}D(\Phi_B)}\right)$$

## S2. Calculation of the effective deformation potential of polar optical phonons

The effective deformation potential is computed by fitting the absorption scattering rate at the minima of the conduction band.

Based on the Fermi golden rule, the scattering rate from an electron state of wave vector $\boldsymbol{k}$ to a state of wave vector $\boldsymbol{k}'$ due to the interaction with a phonon in the branch $\nu$ and wave vector $\boldsymbol{q}$ can be expressed as

$$S_\nu(\boldsymbol{k},\boldsymbol{k}') = \frac{2\pi}{\hbar}\,|g_\nu(\boldsymbol{q})|^2\left(n_{\hbar\omega_\nu(\boldsymbol{q})} + \frac{1}{2} \mp \frac{1}{2}\right)\delta\big(E_{\boldsymbol{k}} - E_{\boldsymbol{k}'} \pm \hbar\omega_\nu(\boldsymbol{q})\big)\,\delta_{\boldsymbol{k},\boldsymbol{k}'\pm\boldsymbol{q}}\,,$$

where $g_\nu(\boldsymbol{q})$ is the matrix element, $\omega_\nu(\boldsymbol{q})$ is the frequency of the phonon, $n_{\hbar\omega_\nu(\boldsymbol{q})}$ is the Bose-Einstein distribution at energy $\hbar\omega_\nu(\boldsymbol{q})$, $E_{\boldsymbol{k}}$ and $E_{\boldsymbol{k}'}$ are the electron energies in the initial and final state, respectively, and the delta functions express the conservations of the energy and the momentum.

The total scattering rate in a state of wave vector $\boldsymbol{k}$ reads

$$\frac{1}{\tau_{LO}(\boldsymbol{k})} = \frac{A}{4\pi^2}\int d\boldsymbol{k}'\, S_{LO}(\boldsymbol{k},\boldsymbol{k}')$$

$$= \frac{2\pi}{\hbar}\frac{A}{4\pi^2}\int d\boldsymbol{k}'\,|g_{LO}(\pm(\boldsymbol{k}-\boldsymbol{k}'))|^2\left(n_{\hbar\omega_{LO}} + \frac{1}{2} \mp \frac{1}{2}\right)\delta(E_{\boldsymbol{k}} - E_{\boldsymbol{k}'} \pm \hbar\omega_{LO})\,, \qquad (2)$$

where the subscript "LO" indicates that longitudinal optical phonons are considered, and a dispersionless approximation has been adopted. Close to a conduction band minimum, the band structure of $CrI_2$ can be described within an effective mass approximation:

$$E(\boldsymbol{k}) = \frac{\hbar^2 {k_x}^2}{2m_x} + \frac{\hbar^2 {k_y}^2}{2m_y}\,, \qquad (3)$$

where $m_x$ and $m_y$ are the effective masses in the transport and in the transverse direction, respectively.

By using the property of the delta function $\delta\big(f(x)\big) = \sum_{x_n}\frac{\delta(x-x_n)}{|f'(x_n)|}$, where $f' = df/dx$, the $x_n$'s are the roots of $f$, and considering the limit $\boldsymbol{k} \longrightarrow \boldsymbol{0}$ in Eq. (3) and the case of phonon absorption, Eq. (2) becomes

$$\frac{1}{\tau_{LO}(\mathbf{0})} =$$
$$= \frac{A}{2\pi\hbar}\frac{2\sqrt{m_x m_y}}{\hbar^2} n_{\hbar\omega_{LO}} \int_{-\sqrt{\hbar\omega_{LO}}}^{\sqrt{\hbar\omega_{LO}}} dq'_y \frac{\left|g_{LO}(\pm(\boldsymbol{k}-\widehat{\boldsymbol{k}}^{+}))\right|^2 + \left|g_{LO}(\pm(\boldsymbol{k}-\widehat{\boldsymbol{k}}^{-}))\right|^2}{2\sqrt{\hbar\omega_{LO} - q'^2_y}}, \quad (4)$$

where $\widehat{\boldsymbol{k}}^{\pm} = \left(\pm\frac{\sqrt{2m_x}}{\hbar}\sqrt{\mp\hbar\omega_{LO} - q'^2_y}, \frac{\sqrt{2m_y}}{\hbar}q'_y\right)$ and $q'_y = \frac{\hbar}{\sqrt{2m_y}}k'_y$.

In order to proceed further, we need to evaluate the matrix element $g_{LO}$. To this purpose, we refer to the model developed in Refs. [2, 3], which is able to account for the screening induced by the dielectric environment. Particularly, we assume the matrix element of the form

$$g_{LO}(\boldsymbol{q}) = \frac{C_Z}{\varepsilon^0_{eff} + r_{eff}|\boldsymbol{q}|} \quad (5)$$

where

$$C_Z = \frac{\sqrt{\hbar}}{4\pi\varepsilon_0}\frac{2\pi {q_e}^2}{A}\sum_a \frac{\boldsymbol{e}_{\boldsymbol{q}_p}\cdot Z^m_a \cdot \boldsymbol{e}^a_{\boldsymbol{q}_p\mathrm{LO}}}{\sqrt{2M_a\omega_{\boldsymbol{q}_p\mathrm{LO}}}}.$$

The quantities $\varepsilon^0_{\mathrm{eff}}$ and $r_{\mathrm{eff}}$ are functions of the dielectric permittivity of the monolayer and of the surrounding materials. Their definitions are provided in Ref. [3].

In the expression of $C_Z$, $\boldsymbol{e}_{\boldsymbol{q}_p}$ denotes the unit vector in the $\boldsymbol{q}$ direction, $\boldsymbol{e}^a_{\boldsymbol{q}_p\mathrm{LO}}$ are the phonon eigenvectors for the branch of interest normalized over the unit cell, $Z^m_a$ is the Born effective charge tensor, $M$ is the atomic mass, and $a$ indexes the atoms within the unit cell. Since the formula assumes that the 2D material has an isotropic dielectric permittivity tensor, we discarded the relatively small deviations from isotropy in $CrI_2$ and we used an average value of $\varepsilon_{\parallel}(0) = 8.5\ \varepsilon_0$ and $\varepsilon_{\parallel}(\infty) = 6.5\ \varepsilon_0$ for the in-plane static and high-frequency dielectric constants, respectively. We made the same approximation for the Born effective charge tensor, which allows us to write

$$C_Z = \frac{\sqrt{\hbar}}{4\pi\varepsilon_0}\frac{2\pi {q_e}^2}{A}\sum_a \frac{Z^m_a \boldsymbol{e}_{\boldsymbol{q}_p}\cdot \boldsymbol{e}^a_{\boldsymbol{q}_p\mathrm{LO}}}{\sqrt{2M_a\omega_{\boldsymbol{q}_p\mathrm{LO}}}} = \frac{\sqrt{\hbar}}{4\pi\varepsilon_0}\frac{2\pi {q_e}^2}{A}\sum_a \frac{Z^m_a \left|\boldsymbol{e}^a_{\boldsymbol{q}_p\mathrm{LO}}\right|}{\sqrt{2M_a\omega_{\boldsymbol{q}_p\mathrm{LO}}}},$$

where the second equality is obtained by considering that phonons in a longitudinal branch propagate in the same direction as $\boldsymbol{q}$. By using the normalization condition $\sum_k \boldsymbol{e}^*_{k\nu}(\boldsymbol{q})\cdot \boldsymbol{e}_{k\nu}(\boldsymbol{q}) = 1$ for the phonon eigenvalues, we can further simplify the expression of $C_Z$ by approximating $\left|\boldsymbol{e}^a_{\boldsymbol{q}_p\mathrm{LO}}\right| \approx 1/\sqrt{N_a}$, where $N_a$ is the total number of atoms in the unit cell.

Thus, we finally obtain

$$g_{LO}(\boldsymbol{q}) \approx \frac{1}{\varepsilon_{eff}^{0} + r_{eff}|\boldsymbol{q}|} \frac{\sqrt{\hbar}}{4\pi\varepsilon_0} \frac{2\pi q_e{}^2}{A} \sum_a \frac{Z_a^m}{\sqrt{2N_a M_a \omega_{\boldsymbol{q}_{pLO}}}} . \tag{6}$$

By using Eq. (6), Eq. (4) can be rewritten as

$$\frac{1}{\tau_{LO}(\boldsymbol{0})} =$$

$$= \frac{A}{2\pi\hbar} \frac{2\sqrt{m_x m_y}}{\hbar^2} n_{\hbar\omega_{LO}} \int_{-\sqrt{\hbar\omega_{LO}}}^{\sqrt{\hbar\omega_{LO}}} dq_y' \frac{1}{2\sqrt{\hbar\omega_{LO} - q_y'^2}} \frac{2C_Z^2}{\left[\varepsilon_{\text{eff}}^0 + r_{\text{eff}}\sqrt{2m_x\hbar\omega_{LO} + (2m_y - 2m_x)q_y'^2}\right]^2}$$

$$\approx \frac{A}{2\pi\hbar} \frac{2\sqrt{m_x m_y}}{\hbar^2} n_{\hbar\omega_{LO}} \int_{-\sqrt{\hbar\omega_{LO}}}^{\sqrt{\hbar\omega_{LO}}} dq_y' \frac{1}{\sqrt{\hbar\omega_{LO} - q_y'^2}} \frac{4\,\hbar^2 C_Z^2}{r_{\text{eff}}{}^2\left(m_x\hbar\omega_{LO} + (4m_y - m_x)q_y'^2\right)}$$

$$= \frac{A}{2\pi\hbar} \frac{2\sqrt{m_x m_y}}{\hbar^2} \frac{4\,\hbar^2 C_Z^2}{r_{\text{eff}}{}^2} \frac{1}{2\sqrt{m_x m_y}\,\hbar\omega_{LO}} n_{\hbar\omega_{LO}} \tan^{-1}\left(\sqrt{\frac{m_y}{m_x}} \frac{2q_y'}{\sqrt{\hbar\omega_{LO} - q_y'^2}}\right)\Bigg|_{-\sqrt{\hbar\omega_{LO}}}^{\sqrt{\hbar\omega_{LO}}}$$

$$= \frac{2\,A\,n_{\hbar\omega_{LO}}}{r_{\text{eff}}{}^2\hbar^2\omega_{LO}} C_Z^2 \approx \frac{n_{\hbar\omega_{LO}} q_e{}^4\hbar}{4\,A(\varepsilon_0 r_{\text{eff}})^2\hbar^2\omega_{LO}^2 N_{at}} \left(\sum_a \frac{Z_a^m}{\sqrt{M_a}}\right)^2 .$$

By considering that in the transistor the monolayer of $CrI_2$ is stacked between the top and bottom $HfO_2$ gate insulators, and by assuming a value of 25 for the dielectric constant of $HfO_2$, we obtain $1/\tau_{LO}(\boldsymbol{0}) \approx 5 \times 10^{10}$ $s^{-1}$.

The deformation potential is obtained from the equation

$$\frac{1}{\tau_{LO}(\boldsymbol{0})} = \frac{D_{OP}^2}{\rho\,\omega_{LO}} \left(\frac{1}{2} \frac{\sqrt{m_x m_y}}{\pi\,\hbar^2}\right) n_{\hbar\omega_{LO}},$$

which expresses the equality between the expression of the absorption scattering rate within the self-consistent Born approximation and the estimated value $1/\tau_{LO}(\boldsymbol{0})$.

By using $m_x = 0.5\,m_0$, $m_y = 5.6\,m_0$, $\hbar\omega_{LO} = 25$ meV, $\rho = 3.3 \times 10^{-7}$g/cm$^2$, and $A$ =0.31 nm$^2$, we find $D_{POP} \approx 0.4 \times 10^8$ eV/cm.

# References

[1] Y. Meir, N. S. Wingreen "Landauer formula for the current through an interacting electron region", *Phys. Rev. Lett.* **68**, 2512. (1992), doi: 10.1103/PhysRevLett.68.2512.

[2] C. Verdi, F. Giustino "Fröhlich electron-phonon vertex from first principles", *Phys. Rev. Lett.* **115**, 176401 (2015), doi: 10.1103/PhysRevLett.115.176401.

[3] T. Sohier, M. Calandra, F. Mauri "Two-dimensional Fröhlich interaction in transition-metal dichalcogenide monolayers: Theoretical modeling and first-principles calculations", *Phys. Rev. B* **94**, 085415 (2016), doi: 10.1103/PhysRevB.94.085415.
